# Supplementary material for: On the Potential of Zines as a Medium for Visualization
Source: arXiv:2108.02177 source file (2021-08-04)
Supplement: Supplementary file 1 [file vis-short-supplement.pdf]

## A SUPPLEMENTARY MATERIALS

In this appendix we provide additional details about various aspects of the work that were unable to fit in the main paper.

### A.1 Survey

In order to better understand the student experience of the zine project during our course we conducted a post-course survey. We draw quotes from this survey in the main body of the text. This Google Forms-hosted survey was conducted 2 months after the course. Students who participated were paid \$6. A reproduction of the study instrument can be found below. Unless otherwise noted each of the responses was configured to be a paragraph style input box. The survey was conducted non-anonymously (in order to verify payment information), and then was anonymized prior to analysis.

1. Prior to the course how familiar were you with zines?

|            |                       |                       |                       |                       |                       |            |
|------------|-----------------------|-----------------------|-----------------------|-----------------------|-----------------------|------------|
| Completely | 1                     | 2                     | 3                     | 4                     | 5                     | Completely |
| Unfamiliar | <input type="radio"/> | <input type="radio"/> | <input type="radio"/> | <input type="radio"/> | <input type="radio"/> | Familiar   |

2. Prior to the course how familiar were you with visualization?

|            |                       |                       |                       |                       |                       |            |
|------------|-----------------------|-----------------------|-----------------------|-----------------------|-----------------------|------------|
| Completely | 1                     | 2                     | 3                     | 4                     | 5                     | Completely |
| Unfamiliar | <input type="radio"/> | <input type="radio"/> | <input type="radio"/> | <input type="radio"/> | <input type="radio"/> | Familiar   |

3. Did you produce a zine for your submission?

- ☐ Yes
- ☐ My submission could have been debatably called a zine.
- ☐ No
- ☐ I'm not sure

4. If you chose to make a zine, why did you pick that format? If not, why not? Did you have prior zine-making experience?

5. Considering both your own work and that of your classmates, do you think zines are a useful medium for visualization? If so, what aspects of zines are conducive to forming visualization narratives? If not, why not?

6. Compare the process of making your printable submission to independent or group projects in other classes. Did you find it more engaging or feel a greater sense of ownership than with other similar projects? Did the process of preparing a printable object change your relationship with your topic?

7. Which tools did you use to create your submission? Please describe your experience using these tools. What was difficult? What was easy? Are there any features you wish existed as part of this combination of tools?

8. If you produced a zine, did you enjoy making the zine making process? Do you think you will make zines again? Do you believe that the process of making this zine will have value for your personal development or your career?

9. Is there anything else you wish to share with us?

Out of the 28 students who took the class, a total of 7 students responded to the survey. Thus, we do not report aggregate statistics as they would only reflect those who elected to participate, and not necessarily the character of the class as a whole.

We sought permission from several students to include their projects in this work (specifically in Fig. 2). Students who allowed us to reproduce their work in this paper were paid \$25.

### A.2 Zine Survey Listing

In Table 1 we list the zines that appeared in our survey. This selection of zines was found by consulting zine librarians, zine bookstores, online archives (such as Issuu and archive.org), and institutional zine archives. There are, of course, additional zines that would be appropriate to consider in this survey, however we did not encounter them. There were a number of zines featuring visualizations that we became aware of but were not able to obtain or view, and hence do not appear in this listing. The intent of this survey was to establish the existence of examples of zines using visualization have come about naturally. Thus while a total survey of zines using visualization is out of scope of this work, we are able to demonstrate that examples do in fact exist.

### A.3 Example Zine

We include a full page version of the example zine shown in Fig. 1 on the final page of this supplement, such that interested parties can print it for themselves, and thus be provided an example of a zine using visualization. It follows standard conventions for constructing a single-page single-sided 8 page zine. Instructions for preparation can be found in various locations online, such as <https://www.wikihow.com/Make-a-Zine>.

Table 1: A listing of the zines that appeared in our sample, along with how they were categorized in our usage theming. Terse names are used in the interest of presentation, but they correspond to the usage themes listed in Sec. 3.

| Zine name and citation |                                                                                                                   | Uses vis. | About data | About vis. | About you | Aligned in form |
|------------------------|-------------------------------------------------------------------------------------------------------------------|-----------|------------|------------|-----------|-----------------|
| Counts                 |                                                                                                                   | 44        | 18         | 5          | 8         | 3               |
| 1                      | Aarati Akkapeddi. <i>Encoding</i> . Undated                                                                       | Yes       | Yes        | No         | Yes       | No              |
| 2                      | Andrew McNutt. <i>Design and analysis of table cartograms</i> . 2019                                              | Yes       | No         | Yes        | No        | No              |
| 3                      | Anna Jo Beck. <i>Biff Boff Bam Sock #8: For your health</i> . 2019                                                | Yes       | No         | No         | No        | No              |
| 4                      | Annie Schleser. <i>perfect!</i> . 2009                                                                            | Yes       | No         | No         | No        | No              |
| 5                      | Anti-eviction mapping project. <i>(Dis)location Black Exodus</i> . 2019                                           | Yes       | Yes        | No         | No        | No              |
| 6                      | Brett Bloom / BKDN BKDN. <i>BREAK DOWN WORKBOOK #2—SONIC MEDITATIONS: INVESTIGATING PETRO-SUBJECTIVITY</i> . 2019 | Yes       | No         | No         | No        | No              |
| 7                      | Bubblesort Zines. <i>Hip-Hip Array</i> . 2016                                                                     | Yes       | No         | No         | No        | No              |
| 8                      | Carni Klirs. <i>Visualizing the History of Fugazi</i> . 2018                                                      | Yes       | Yes        | No         | No        | Yes             |
| 9                      | Cecilia Zhao. <i>GARBAGE</i> . 2019                                                                               | Yes       | Yes        | No         | No        | No              |
| 10                     | Charlotte Francoeur, Lindsey Leigh. <i>The Wonderful World of Microbes Written</i> . 2021                         | Yes       | Yes        | No         | No        | No              |
| 11                     | Corinne Halbert, Erika Iris and Demi Zigler. <i>Mathematics for Misfits</i> . 2021                                | Yes       | No         | No         | No        | No              |
| 12                     | Equity and Health Innovations Design Research Lab. <i>The Denizen Designer Zine</i> . 2021                        | Yes       | Yes        | No         | No        | No              |
| 13                     | FAQNP: A Queer Nerd Publication. <i>Queer Nerds Visualized</i> . 2014                                             | Yes       | No         | No         | Yes       | No              |
| 14                     | Gabe Wigtil. <i>The Solar System to Scale - science astronomy mini zine</i> . Undated                             | Yes       | No         | No         | No        | No              |
| 15                     | Hannah Israelsohn. <i>Language Zine</i> . 2008                                                                    | Yes       | No         | No         | No        | No              |
| 16                     | Joe Song. <i>Awesome Attributes About Ants</i> . 2009                                                             | Yes       | No         | No         | No        | No              |
| 17                     | Joe Song. <i>The beginner's guide to variable stars</i> . Undated                                                 | Yes       | No         | No         | No        | No              |
| 18                     | Joe Song. <i>The beginner's guide to binary stars</i> . Undated                                                   | Yes       | No         | No         | No        | No              |
| 19                     | Johnny Masiuleqicz. <i>Happy Tapir #3 A cup of holiday fear</i> . 2017                                            | Yes       | No         | No         | Yes       | No              |
| 20                     | Jupiter Hadley and Dann Sullivan. <i>Seeds</i> . 2016-                                                            | Yes       | Yes        | No         | No        | No              |
| 21                     | Lilian Huang. <i>I can't explain it any other way': a zine of Lilian's concert attendance, 2019, 2020</i>         | Yes       | Yes        | No         | Yes       | No              |
| 22                     | Lily Xie. <i>Charts</i> . Undated                                                                                 | Yes       | No         | No         | Yes       | No              |
| 23                     | Liz Mason. <i>Most Unwanted Zine</i> . 2021                                                                       | Yes       | Yes        | No         | No        | Yes             |
| 24                     | luxoft. <i>Tech Spark</i> . 2021                                                                                  | Yes       | No         | Yes        | No        | No              |
| 25                     | Melissa Simerson. <i>Superfoods</i> . Undated                                                                     | Yes       | Yes        | No         | No        | No              |
| 26                     | Papercuts library. <i>#2: Results of the longest bull market in american history</i> . 2020                       | Yes       | Yes        | No         | No        | No              |
| 27                     | Patrice Solomon, Jarad Solomon. <i>A science of mind and non-physical realms</i> . 2019                           | Yes       | No         | No         | No        | No              |
| 28                     | Pocket Lint. <i>Pocket Lint's Party Zine Spring 2018</i> . 2018                                                   | Yes       | No         | No         | No        | No              |
| 29                     | Pocket Lint. <i>Crying on Campus</i> . Undated                                                                    | Yes       | Yes        | No         | No        | No              |
| 30                     | REDACTED. <i>On the Potential of Zines as a Medium for Visualization</i> . 2021                                   | Yes       | No         | Yes        | No        | Yes             |
| 31                     | Rolling Thunder: An Anarchist Journal of Dangerous Living. <i>Rolling Thunder 10 (Summer 2012)</i> . 2012         | Yes       | No         | No         | No        | No              |
| 32                     | Sarah McNeil. <i>Statistical Things That Happen But Don't Matter</i> . 2011                                       | Yes       | No         | No         | Yes       | No              |
| 33                     | Sarah McNeil. <i>Updated Report of Observations Which Somehow Seem to Reflect Abstractly on Life</i> . 2011       | Yes       | No         | No         | Yes       | No              |
| 34                     | Sarah Poppy Jackson. <i>Reclaim your sh*t!</i> . 2019                                                             | Yes       | Yes        | No         | No        | No              |
| 35                     | The Sophie Lab. <i>Newcomb tech in mind: the zine of of newcomb's institute of technology</i> . 2018-             | Yes       | Yes        | Yes        | No        | No              |
| 36                     | Tim Devin. <i>Mapping out utopia: 1970s Boston-area counterculture</i> . 2017                                     | Yes       | Yes        | No         | No        | No              |
| 37                     | Tina Richardson. <i>Stepz: a psychogeography and urban aesthetics zine</i> . 2015                                 | Yes       | No         | No         | No        | No              |
| 38                     | Tiziana Alocci, Piero Zagami. <i>Market cafe magazine</i> . 2017 -                                                | Yes       | No         | Yes        | No        | No              |
| 39                     | Tom Vague. <i>Vague 28: Wild West 11</i> . 1997                                                                   | Yes       | No         | No         | No        | No              |
| 40                     | Two Photon Art. <i>Nicotine Zine</i> . 2019                                                                       | Yes       | Yes        | No         | No        | No              |
| 41                     | Two Photon Art. <i>The Opium Poppy</i> . 2016                                                                     | Yes       | Yes        | No         | No        | No              |
| 42                     | Two-Fisted Library Studies. <i>Volume 8, Number 1</i> . 2017                                                      | Yes       | No         | No         | No        | No              |
| 43                     | Unknown. <i>Fuck solitary: abolition &amp; HB5417</i> . Undated                                                   | Yes       | No         | No         | Yes       | No              |
| 44                     | Victoria Harley, Katrina Eresman. <i>Terrific trees of the USA!</i> . Undated                                     | Yes       | Yes        | No         | No        | No              |

# On the Potential of Zines as a Medium for Visualization

## A zine about a paper about zines using data visualization

By <REDACTED>

### What is a zine?

This is a zine! But if you want a more formal definition:

Zines are non-commercial, non-professional, small-circulation magazines which their creators produce, publish, and distribute by themselves

- Duncombe

They come in all shapes and sizes. Some (just a couple of pages or a couple of inches big) are small, some are large. They appear in (hundreds of pages and figures!) forms that are familiar and forms that are weird. They are often only available in the physical world, but sometimes they're collected online. (such as Issuu and archive.org)

Anyone can make a zine. They can be produced using high-end digital tools as well as with juxtaposed pieces of paper and a photocopier. This makes them accessible to everyone!

## Despite these enticing features there has been little work in vis👁️zines!

### Narrative Visualization

### Zines

vis👁️zines! << [zines]  
[vis👁️zines] << [vis]

Zines seem to be a natural place for vis work, as their intimate physical form offers a range of affordances that are advantageous to vis. But there hasn't been any scholarship and there has been relatively limited practice. In this zine we argue that **zines should be seen as a viable medium for visualization**.

At least that's our belief! Zines are often purely physical objects and so it's difficult to completely survey their usage

## Read the paper or visit (REDACTED) to find out more!

### On the Potential of Zines as a Medium for Visualization

ANON AUTHORS

Abstract

Visualization is considered a rich way of presenting, analyzing, and communicating data. Zines are often purely physical objects and so it's difficult to completely survey their usage. This paper explores the potential of zines as a medium for visualization. It opens the door to interesting questions such as: Zines are often told from the first person; how does this affect the way that people trust data displays in that mode? Zinesters often have rich knowledge about particular topics and ways of expressing themselves about those topics, which would seem to make them ideal collaborators for data projects.

1. Introduction

Visualizations are considered a rich way of presenting, analyzing, and communicating data. Zines are often purely physical objects and so it's difficult to completely survey their usage. This paper explores the potential of zines as a medium for visualization. It opens the door to interesting questions such as: Zines are often told from the first person; how does this affect the way that people trust data displays in that mode? Zinesters often have rich knowledge about particular topics and ways of expressing themselves about those topics, which would seem to make them ideal collaborators for data projects.

2. Related Work

This paper explores the potential of zines as a medium for visualization. It opens the door to interesting questions such as: Zines are often told from the first person; how does this affect the way that people trust data displays in that mode? Zinesters often have rich knowledge about particular topics and ways of expressing themselves about those topics, which would seem to make them ideal collaborators for data projects.

## Observations

In our class and in our search we found several **design patterns** that are unusual among forms that vis typically appears in, including

- Zine's accessibility helps **Surface**
- Other Voices** that might not normally find a venue for their perspectives.

Their printed form **Imparts an Intimacy** that can help build community and offer a foundation to talk about difficult topics.

Data is often seen as objective. Zines can help this **Shatter the View from Nowhere** by locating the author and the works provenance as a prominent part of their design.

## We explored vis👁️zines in a recent class project

In a recent class on Data Vis for Public Policy Course students were allowed to make zines about policy topics for a project. A majority of the students made zines for the project, and spoke positively about the experience.

**Student comments:**

"The ability to order visualizations sequentially or thematically, and to accompany them with text, gives you a lot of control over the narrative structure, and I think zines come with audience expectations of being a mélange, so you can have a diversity of visualization types instead of cleaving so strictly to a single polished (and more bland) house style."

"Being able to turn pages like a book so that certain visualizations are hidden can help drive story-telling"

"Made me think about the position and description of graphs and how they connect to previous/next pages."

"I really enjoyed the process [of zine making] - I found it easy to build the narrative through the process and felt able to communicate what I wanted to communicate through my zine."

project breakdown

| Category | Count |
|----------|-------|
| Zine     | 16    |
| Other    | 8     |
| Maybe    | 5     |

## 44 zines that use visualization in some way

To understand the potential of this combination we sought out zines with visualizations

By searching we identified

- online zine repositories
- bookstores and zine fairs
- institutional archives

We coded the way that vis is used in each zine. There are doubtless other reasons to use vis in a zine beyond these—our sample was limited by social distancing, and favored examples found online—but we believe these are evocative of the general case.

This excludes the zines students made in our classes, as we wanted to establish that this the intersection of vis and zines is occupied in the wild.

(see next page)

Although there are definitely more! Our search was meant to show that the intersection is not empty

Zines about visualization

Zines seem to address every conceivable topic, vis included. **Market Cafe Mag** is a prominent of this style of usage, (despite being a series, we only count it once)

Zines about data

Zines can be used to tell complex data stories in a friendly and accessible way. This can involve classic-zine practice of list making, as well as usages like advocacy and activism through maps and charts, such as in the splendid **(Dis)location Black Exodus** from AEMP.

Zines using visualization

Similar to many other mediums, sometimes zines just use vis to enforce their points.

Zines about you

The perzine genre is ubiquitous among zines and connects with vis in a data humanist style.

Zines aligned in content

Some zines pair well with vis due to alignment in form and content.

hey that's this zine

For instance Kilrs' History of Fugazi
